# Supplementary material for: KRust: A Formal Executable Semantics of Rust
Source: arXiv:1804.10806 source file (2018-04-28)
Supplement: Supplementary file 1 [file appendix.tex]

\onecolumn
\appendix
